# Supplementary material for: Community Detection with Heterogeneous Block Covariance Model
Source: arXiv:2412.03780 source file (2024-12-04)
Supplement: Supplementary file 1 [file c7-appendix.tex]

%%%%%%%%%%%%%%%%%%%%%%%%%%%%%%%%%%%%%%%%%%%%%%%%%%%%%%%%%%%%%%%%%%%%%%%%%%%%%%
% \addcontentsline{toc}{chapter}{Appendix}
% \vspace{5mm} 

% \subsection*{\centerline{Appendix}}

\subsubsection*{A1 Derivation of the variational expectation-maximization algorithm}

In this section, we provide details on the factorization of  $q_1(\V{c}), q_2(\V{\alpha})$ and derivation of parameter estimators in closed-forms involved in the variational EM algorithm. Recall that the algorithm maximizes 
\begin{align*}
 J(q_1(\V{c}),q_2(\V{\alpha}), \Phi) = &\sum_{\V{c} \in \{1,...,K\}^P}\int_{\V{\alpha}\in \mathbb{R}^{N\times K}} q_1(\V{c})q_2( \V{\alpha})L(\M{X},\V{c},\V{\alpha}|\Phi)d\V{\alpha} \\
  & - \sum_{\V{c} \in \{1,...,K\}^P}\int_{\V{\alpha}\in \mathbb{R}^{N\times K}} q_1(\V{c})q_2( \V{\alpha})\log q_1(\V{c})q_2( \V{\alpha}) d\V{\alpha},
\end{align*}
over $q_1(\V{c})$, $q_2(\V{\alpha})$ and $\Phi$ iteratively, 
where 
\begin{align*}
 L(\M{X},\V{c},\V{\alpha}|\Phi)
= & \log \big[f(\V{c}|\V{\pi})f(\V{\alpha}|\bome)f(\M{X}|\V{c},\V{\alpha},\{\lambda_j\}, \{\sigma_j\})\big] \\
= & \sum_{j=1}^P\sum_{k=1}^K 1(c_j=k)\log{\pi_k} -\frac{N}{2}\log|\bome|-\frac{1}{2}\sum_{i=1}^N\V{\alpha}_i^T\bome^{-1}\V{\alpha}_i \\
    &  +  \sum_{j=1}^P\sum_{i=1}^N\sum_{k=1}^K 1(c_j=k)\bigg( -\frac{1}{2}\log\sigma_j^2-\frac{(X_{ij}-\lambda_j\alpha_{ik})^2}{2\sigma_j^2}\bigg).
\end{align*}

\textbf{Proof of factorization $q_1(\V{c})=\prod_{j=1}^P\frac{q_1(c_j)}{\sum_{k=1}^Kq_1(c_j=k)}$ } 

\begin{proposition}
Let
\begin{align*}
    g_1(c_j) = \exp\left\{ \ln \pi_{c_j} +  \sum_{i=1}^N\bigg( -\frac{1}{2}\ln\sigma_j^2-\frac{\mathbb{E}_{q_2}(X_{ij}-\lambda_j\alpha_{ic_j})^2}{2\sigma_j^2}\bigg)\right\}.
\end{align*}
Given $\Phi$ and $q_2(\V{\alpha})$, 
\begin{align*}
\argmax_{q_1} J(q_1,q_2,\Phi)
\end{align*}
is achieved at 
\begin{align}
 q_1(\V{z}) = & \prod_{i=1}^m \frac{ e^{g_1(z_i)} }{ \sum_{k=1}^K  e^{g_1(k)} }. \label{factor1}
\end{align}
\end{proposition}

\begin{proof}
Given $q_2(\V{\alpha})$ and $\Phi$, updating $q_1(\V{c})$ is equivalent to maximizing
\begin{align*}
     J_1(q_1,q_2, \Phi)&=\sum_{\V{c} \in \{1,...,K\}^P}\ q_1(\V{c})\int_{\V{\alpha}\in \mathbb{R}^{N\times K}}q_2( \V{\alpha})L(\M{X},\V{c},\V{\alpha}|\Phi)d\V{\alpha}  - \sum_{\V{c} \in \{1,...,K\}^P} q_1(\V{c})\ln q_1(\V{c}) \\
     & = \sum_{\V{c} \in \{1,...,K\}^P}\ q_1(\V{c})\mathbb{E}_{q_2}(L(\M{X},\V{c},\V{\alpha}|\Phi)) - \sum_{\V{c} \in \{1,...,K\}^P} q_1(\V{c})\ln q_1(\V{c}),
\end{align*}
and up to a constant 
\begin{align*}
   \mathbb{E}_{q_2}(L(\M{X},\V{c},\V{\alpha}|\Phi)) & =\sum_{j=1}^P\sum_{k=1}^K 1(c_j=k)\ln{\pi_k}\\
   & \quad +  \sum_{j=1}^P\sum_{i=1}^N\sum_{k=1}^K 1(c_j=k)\bigg( -\frac{1}{2}\ln\sigma_j^2-\frac{\mathbb{E}_{q_2}(X_{ij}-\lambda_j\alpha_{ik})^2}{2\sigma_j^2}\bigg). 
\end{align*}
Next after rearranging the terms we obtain that
\begin{align*}
\mathbb{E}_{q_2}(L(\M{X},\V{c},\V{\alpha}|\Phi)) & = \sum_{j=1}^P\ln \pi_{c_j} + \sum_{j=1}^P\sum_{i=1}^N\bigg( -\frac{1}{2}\ln\sigma_j^2-\frac{\mathbb{E}_{q_2}(X_{ij}-\lambda_j\alpha_{ic_j})^2}{2\sigma_j^2}\bigg)\\
& =\sum_{j=1}^P\bigg[\ln \pi_{c_j} +  \sum_{i=1}^N\bigg( -\frac{1}{2}\ln\sigma_j^2-\frac{\mathbb{E}_{q_2}(X_{ij}-\lambda_j\alpha_{ic_j})^2}{2\sigma_j^2}\bigg)\bigg]\\
&= \ln \prod_{j=1}^P q_1(c_j),
\end{align*}
where 
\begin{align*}
    q_1(c_j) = \exp\left\{ \ln \pi_{c_j} +  \sum_{i=1}^N\bigg( -\frac{1}{2}\ln\sigma_j^2-\frac{\mathbb{E}_{q_2}(X_{ij}-\lambda_j\alpha_{ic_j})^2}{2\sigma_j^2}\bigg)\right\}.
\end{align*}
Then we have 
\begin{align*}
 J_1(q_1,q_2, \Phi)&= \sum_{\V{c} \in \{1,...,K\}^P}\ q_1(\V{c})\ln \prod_{j=1}^P q_1(c_j) - \sum_{\V{c} \in \{1,...,K\}^P} q_1(\V{c})\ln q_1(\V{c}). \\
 & = \sum_{\V{c} \in \{1,...,K\}^P} q_1(\V{c})\ln \frac{\prod_{j=1}^P q_1(c_j)}{q_1(\V{c})} \\
 & \leq \ln \sum_{\V{c} \in \{1,...,K\}^P}q_1(\V{c})\frac{\prod_{j=1}^P q_1(c_j)}{q_1(\V{c})} \quad \mbox(\text{Jensen's ineqaulity}) \\
 &=\ln \sum_{\V{c} \in \{1,...,K\}^P}\prod_{j=1}^P q_1(c_j)
\end{align*}
The equality holds when $\frac{\prod_{j=1}^P q_1(c_j)}{q_1(\V{c})}$ is constant with respect to  $\V{c}$, i.e.
\begin{align*}
    q_1(\V{c}) & = \frac{\prod_{j=1}^P q_1(c_j)}{\sum_{\V{c}' \in \{1,...,K\}^P}\prod_{j=1}^P q_1(c_j^{'})} \\
    & =\frac{\prod_{j=1}^P q_1(c_j)}{\prod_{j=1}^P(\sum_{k=1}^K q_1(c_j^{'}=k))}\\
    & =\prod_{j=1}^P\frac{q_1(c_j)}{\sum_{k=1}^K q_1(c_j^{'}=k)}
\end{align*}
\end{proof}

\textbf{Proof of factorization $q_2(\V{\alpha})=\prod_{i=1}^N\frac{q_2(\alpha_i)}{\int_{\alpha_i\in \mathbb{R}^K}q_2(\alpha_i)d\alpha_i}$ } 

\begin{proof}
Given $q_1(\V{c})$ and $\Phi$, updating $q_2(\V{\alpha})$ is equivalent to maximizing
\begin{align*}
J_2(q_1,q_2, \Phi)&=\sum_{\V{c} \in \{1,...,K\}^P}\int_{\V{\alpha}\in \mathbb{R}^{N\times K}} q_1(\V{c})q_2( \V{\alpha})L(\M{X},\V{c},\V{\alpha}|\Phi)d\V{\alpha} - \int_{\V{\alpha}\in \mathbb{R}^{N\times K}}q_2( \V{\alpha})\ln q_2( \V{\alpha})d\V{\alpha}\\
& = \int_{\V{\alpha}\in \mathbb{R}^{N\times K}} q_2( \V{\alpha})\mathbb{E}_{q_1}(L(\M{X},\V{c},\V{\alpha}|\Phi))d\V{\alpha}- \int_{\V{\alpha}\in \mathbb{R}^{N\times K}}q_2( \V{\alpha})\ln q_2( \V{\alpha})d\V{\alpha},
\end{align*}
and up to a constant we have
\begin{align*}
\mathbb{E}_{q_1}(L(\M{X},\V{c},\V{\alpha}|\Phi)) & =  -\frac{1}{2}\sum_{i=1}^N\V{\alpha}_i^T\bome^{-1}\V{\alpha}_i   +  \sum_{j=1}^P\sum_{i=1}^N\sum_{k=1}^K \mathbb{E}_{q_1}[1(c_j=k)]\bigg(-\frac{(X_{ij}-\lambda_j\alpha_{ik})^2}{2\sigma_j^2}\bigg).
\end{align*}

Next after rearranging of the terms we obtain that
\begin{align*}
 \mathbb{E}_{q_1}(L(\M{X},\V{c},\V{\alpha}|\Phi)) & =  \sum_{i=1}^N\bigg[-\frac{1}{2} \V{\alpha}_i^T\bome^{-1}\V{\alpha}_i-\frac{1}{2}\sum_{j=1}^P\sum_{k=1}^K\frac{\mathbb{E}_{q_1}[1(c_j=k)]}{\sigma_j^2}(X_{ij}-\lambda_j\alpha_{ik})^2\bigg]\\
 & = \ln\prod_{i=1}^Nq_2(\V{\alpha}_i),
\end{align*}
where
\begin{align*}
    q_2(\V{\alpha}_i) =\exp\left\{-\frac{1}{2} \V{\alpha}_i^T\bome^{-1}\V{\alpha}_i-\frac{1}{2}\sum_{j=1}^P\sum_{k=1}^K\frac{\mathbb{E}_{q_1}[1(c_j=k)]}{\sigma_j^2}(X_{ij}-\lambda_j\alpha_{ik})^2\right\}.
\end{align*}

Then we have
\begin{align*}
    J_2(q_1,q_2, \Phi)&=\int_{\V{\alpha}\in \mathbb{R}^{N\times K}} q_2( \V{\alpha})\ln\prod_{i=1}^Nq_2(\V{\alpha}_i)d\V{\alpha}- \int_{\V{\alpha}\in \mathbb{R}^{N\times K}}q_2( \V{\alpha})\ln q_2( \V{\alpha})d\V{\alpha}\\
    & = \int_{\V{\alpha}\in \mathbb{R}^{N\times K}}q_2( \V{\alpha})\ln \frac{\prod_{i=1}^Nq_2(\V{\alpha}_i)}{q_2( \V{\alpha})}d\V{\alpha}\\
    & \leq \ln\int_{\V{\alpha}\in \mathbb{R}^{N\times K}}\prod_{i=1}^Nq_2(\V{\alpha}_i)d\V{\alpha}.
\end{align*}
The equality holds when $\frac{\prod_{i=1}^Nq_2(\V{\alpha}_i)}{q_2(\V{\alpha})}$ is constant with respect to $\V{\alpha}$, i.e.
\begin{align*}
    q_2(\V{\alpha}) = \frac{\prod_{i=1}^Nq_2(\V{\alpha}_i)}{\int_{\V{\alpha}^{'}\in \mathbb{R}^{N\times K}}\prod_{i=1}^Nq_2(\V{\alpha}_i^{'})d\V{\alpha}'} =\prod_{i=1}^N\frac{q_2(\V{\alpha}_i)}{\int_{\V{\alpha}_i\in \mathbb{R}^K}q_2(\V{\alpha}_i^{'})d\V{\alpha}_i^{'}}.
\end{align*}

Lastly we show that  $q_2(\V{\alpha}_i)$ actually follows a $K$-variate normal distribution.

Let 
\begin{align*}
\M{D}_{j}&= \frac{\lambda_j^2}{\sigma_j^2}\begin{pmatrix}
\mathbb{E}_{q_1}(1(c_j=1)) & 0 & \cdots & 0 \\
0 & \mathbb{E}_{q_1}(1(c_j=2)) & \cdots & 0 \\
\vdots & \vdots & \ddots & \vdots\\
0 & 0 & \cdots & \mathbb{E}_{q_1}(1(c_j=K))
\end{pmatrix}_{K \times K},\\
    \V{b}_{ij} &=\frac{1}{\lambda_j}\begin{pmatrix}
    X_{ij}\\
    X_{ij}\\
    \vdots \\
    X_{ij}
    \end{pmatrix}_{K\times 1},  
\end{align*}

then we can reorganize the exponential terms of $q_2(\V{\alpha}_i)$ as a quadratic function of $\V{\alpha}_i$,
\begin{align*}
Q(\V{\alpha}_i)&= \V{\alpha}_i^T\bome^{-1}\V{\alpha}_i+\sum_{j=1}^P\sum_{k=1}^K\frac{\mathbb{E}_{q_1}[1(c_j=k)]}{\sigma_j^2}(X_{ij}-\lambda_j\alpha_{ik})^2\\
& = \V{\alpha}_i^T\bome^{-1}\V{\alpha}_i+\sum_{j=1}^P(\V{\alpha}_i-\V{b}_{ij})^T \V{D}_j (\V{\alpha}_i-\V{b}_{ij})\\
& \propto \V{\alpha}_i^T\bome^{-1}\V{\alpha}_i +\sum_{j=1}^P\V{\alpha}_i^T \V{D}_j\V{\alpha}_i - \big(\sum_{j=1}^P\V{b}_{ij}^T\V{D}_j\big)\V{\alpha}_i - \V{\alpha}_i^T\big(\sum_{j=1}^P\V{D}_j\V{b}_{ij}\big)\\
& = \V{\alpha}_i^T\big(\bome^{-1}+\sum_{j=1}^P\V{D}_j\big)\V{\alpha}_i - \big(\sum_{j=1}^P\V{b}_{ij}^T\V{D}_j\big)\V{\alpha}_i - \V{\alpha}_i^T\big(\sum_{j=1}^P\V{D}_j\V{b}_{ij}\big)
\end{align*}

Let $\V{A}=\bome^{-1}+\sum_{j=1}^P\V{D}_j$ and $\V{B}_i=\sum_{j=1}^P\V{D}_j\V{b}_{ij}$,
\begin{align*}
 Q(\V{\alpha}_i)&\propto  \V{\alpha}_i^T \V{A}\V{\alpha}_i - \V{B}_i^T\V{\alpha}_i -\V{\alpha}_i^T\V{B}_i + \V{B}_i^T\V{A}^{-1}\V{B}_i\\
 & = \V{\alpha}_i^T \V{A}\V{\alpha}_i - \V{B}_i^T\V{A}^{-1}\V{A}\V{\alpha}_i -\V{\alpha}_i^T\V{A}\V{A}^{-1}\V{B}_i + \V{B}_i^T\V{A}^{-1}\V{A}\V{A}^{-1}\V{B}_i
\end{align*}

Let $\V{V}=\V{A}^{-1}$ and $\V{\mu}_i=\V{A}^{-1}\V{B}_i$, then
\begin{align*}
     Q(\V{\alpha}_i)&\propto (\V{\alpha}_i-\V{\mu}_i)^T\V{V}^{-1}(\V{\alpha}_i-\V{\mu}_i)
\end{align*}

Therefore $q_2(\V{\alpha}_i)$ follows $K$-variate normal distribution $N(\V{\mu}_i, \V{V})$.
\end{proof}

\textbf{Proof of parameter estimators in closed-form}

\begin{proof}
Given $q_1(\V{c})$ and $q_2(\V{\alpha})$, updating $\Phi$ is equivalent to maximizing
\begin{align*}
    J_3(q_1,q_2, \Phi)&=\sum_{\V{c} \in \{1,...,K\}^P}\int_{\V{\alpha}\in \mathbb{R}^{N\times K}} q_1(\V{c})q_2( \V{\alpha})L(\M{X},\V{c},\V{\alpha}|\Phi)d\V{\alpha}\\
    & = \mathbb{E}_{q_1 \times q_2}(L(\M{X},\V{c},\V{\alpha}|\Phi))
\end{align*}

\begin{enumerate}
    \item Optimizer of $\V{\pi}$.
    
    Up to a constant we have
    \begin{align*}
        J_3(q_1,q_2, \Phi)&= \sum_{j=1}^P\sum_{k=1}^K\mathbb{E}_{q_1}[1(c_j=k)]\ln \pi_k \quad \text{s.t} \quad  \sum_{k=1}^K \pi_k=1.
    \end{align*}
    
With Lagrange multiplier, the Lagrange function becomes
\begin{align*}
    \text{Lag}(\gamma, \V{\pi}) & = \sum_{j=1}^P\sum_{k=1}^K\mathbb{E}_{q_1}[1(c_j=k)]\ln \pi_k + \gamma(1-\sum_{k=1}^K \pi_k)
\end{align*}
Take derivative w.r.t $\pi_k$,
\begin{align*}
    \frac{\partial \text{Lag}(\gamma, \V{\pi})}{\partial \pi_k} &= \frac{\sum_{j=1}^P\mathbb{E}_{q_1}[1(c_j=k)]}{\pi_k} - \gamma
\end{align*}
Then
\begin{align*}
\frac{\partial \text{Lag}(\gamma, \V{\pi})}{\partial \pi_k} = 0 & \Rightarrow \gamma\pi_k =\sum_{j=1}^P\mathbb{E}_{q_1}[1(c_j=k)]\\
& \Rightarrow \gamma =\sum_{k=1}^K\sum_{j=1}^P\mathbb{E}_{q_1}[1(c_j=k)]\\
& \Rightarrow \hat{\pi}_k = \frac{\sum_{j=1}^P \mathbb{E}_{q_1}[1(c_j=k)]}{\sum_{j=1}^P\sum_{k'=1}^K \mathbb{E}_{q_1}[1(c_j=k')]}.
\end{align*}

\item Optimizer of $\bome$.

Up to a constant we have
\begin{align*}
     J_3(q_1,q_2, \Phi)&=-\frac{N}{2}\ln |\bome| -\frac{1}{2}\sum_{i=1}^N\mathbb{E}_{q_2}(\V{\alpha}_i^T\bome^{-1}\V{\alpha}_i). 
\end{align*}
Since $J_3(q_1,q_2, \Phi)$ is the log-likelihood of a $K$-variate normal distribution up to a constant, the maximum-likelihood estimator of $\bome$ is the sample covariance $\hat{\bome} = \frac{1}{N}\sum_{i=1}^N\mathbb{E}_{q_2}(\V{\alpha}_i\V{\alpha}_i^T)$.

\item Optimizer of $\{\lambda_j\}$ and $\{\sigma_j^2\}$.

Up to a constant we obtain
{\small
\begin{align*}
J_3(q_1,q_2, \Phi)&= \sum_{j=1}^P\sum_{i=1}^N\sum_{k=1}^K\mathbb{E}_{q_1}[1(c_j=k)]\bigg( -\frac{1}{2}\ln\sigma_j^2-\frac{(X_{ij}^2+\lambda_j^2\mathbb{E}_{q_2}[\alpha_{ik}^2]-2\lambda_j\mathbb{E}_{q_2}[\alpha_{ik}])}{2\sigma_j^2}\bigg)
\end{align*}
}
Take derivative w.r.t $\lambda_j$ and set the score equation equal to zero gives
\begin{align*}
   \hat{\lambda}_j & = \frac{\sum_{i=1}^N\sum_{k=1}^K \mathbb{E}_{q_1}[1(c_j=k)]X_{ij}\mathbb{E}_{q_2}[\alpha_{ik}]}{\sum_{i=1}^N\sum_{k=1}^K \mathbb{E}_{q_1}[1(c_j=k)]\mathbb{E}_{q_2}[\alpha_{ik}^2]} \quad  
\end{align*}
Similarly, take derivative w.r.t to $\sigma_j^2$ and set the score equation equal to zero gives
\begin{align*}
    \hat{\sigma}_j^2 & = \frac{\sum_{i=1}^N\sum_{k=1}^K \mathbb{E}_{q_1}[1(c_j=k)]
    \mathbb{E}_{q_2}(X_{ij}^2+\hat{\lambda}_j^2\alpha_{ik}^2-2\hat{\lambda}_jX_{ij}\alpha_{ik})}{N} .
\end{align*}
\end{enumerate}

\end{proof}

\subsubsection*{A2 Proof of Proposition 1}

\begin{proposition*}
 $\bar{J}(\bqc, \bqa; \Phi^*)$ has an unique optimizer achieved at $\bqc = \bic, \bqa = \balp^*$, up to the community permutation.
\end{proposition*}

\begin{proof}
Given the model assumption of $X_{ij}=\lambda_j \alpha_{ic_j}+ \sigma_j \epsilon_{ij}$,  the conditional mean and second moment of $X_{ij}$ are
\begin{align*}
    & \mathbb{E}(X_{ij}|\balp^*,\V{c}^*) = \lambda_j^{*}\alpha^*_{ic_j} \\
    & \mathbb{E}(X_{ij}^2|\balp^*,\V{c}^*) = \sigma_j^{*2} + \lambda_j^{*2}\alpha^{*2}_{ic_j}.
\end{align*}
And $\bar{J}(\bqc, \bqa; \Phi^*)$ and $\bar{J}(\bic, \balp^*; \Phi^*)$ can be written as 
\begin{align*}
    & \bar{J}(\bqc, \bqa; \Phi^*) \\
    & = -\sum_{i=1}^N\sum_{j=1}^P\frac{\sigma_j^{*^2} +\lambda_j^{*^2}(\sum_{k=1}^KI_{jk}^c\alpha_{ik}^{*^2})}{2\sigma_j^{*2}} - \sum_{i=1}^N\sum_{j=1}^P\sum_{k=1}^K\frac{\lambda_j^{*2}q_{jk}^cq_{ik}^{\alpha^2}}{2\sigma_j^{*2}}\\
    & \quad + \sum_{i=1}^N\sum_{j=1}^P\sum_{k=1}^K\frac{\lambda_j^{*2}q_{jk}^cq_{ik}^{\alpha}(\sum_{k'=1}^KI_{jk'}^c\alpha_{ik'}^{*})}{\sigma_j^{*2}}\\
  & \bar{J}(\bic, \balp^*; \Phi^*)\\
  & = -\sum_{i=1}^N\sum_{j=1}^P\frac{\sigma_j^{*^2} +\lambda_j^{*^2}(\sum_{k=1}^KI_{jk}^c\alpha_{ik}^{*^2})}{2\sigma_j^{*2}} - \sum_{i=1}^N\sum_{j=1}^P\sum_{k=1}^K\frac{\lambda_j^{*2}I_{jk}^c\alpha_{ik}^{*^2}}{2\sigma_j^{*2}}\\
    & \quad + \sum_{i=1}^N\sum_{j=1}^P\sum_{k=1}^K\frac{\lambda_j^{*2}I_{jk}^c\alpha_{ik}^*(\sum_{k'=1}^KI_{jk'}^c\alpha_{ik'}^{*})}{\sigma_j^{*2}}.
\end{align*}
Take the difference between $\bar{J}(\bqc, \bqa; \Phi^*)$ and $\bar{J}(\bic, \balp^*; \Phi^*)$, we have
\begin{align*}
& \bar{J}(\bic, \balp^*; \Phi^*) -  \bar{J}(\bqc, \bqa; \Phi^*) \\
& = \sum_{i=1}^N\sum_{j=1}^P\sum_{k=1}^K\frac{\lambda_j^{*2}}{\sigma_j^{*2}}\left(\frac{1}{2}(q_{jk}^cq_{ik}^{\alpha^2}-I_{jk}^c\alpha_{ik}^{*^2})\right)   \\
& \quad + \sum_{i=1}^N\sum_{j=1}^P\sum_{k=1}^K\frac{\lambda_j^{*2}}{\sigma_j^{*2}}\left((\sum_{k'=1}^KI_{jk'}^c\alpha_{ik'}^{*})(I_{jk}^c\alpha_{ik}^{*} - q_{jk}^cq_{ik}^{\alpha})\right) \\
& = \sum_{i=1}^N\sum_{j=1}^P\frac{\lambda_j^{*^2}}{\sigma_j^{*^2}}\bigg[\frac{1}{2}(\sum_{k'=1}^KI_{jk'}^c\alpha_{ik'}^{*^2}) + \frac{1}{2}(\sum_{k=1}^Kq_{jk}^cq_{ik}^{\alpha^2}) - (\sum_{k'=1}^KI_{jk'}^c\alpha_{ik'}^{*})(\sum_{k=1}^Kq_{jk}^cq_{ik}^{\alpha})\bigg] \\
& =\sum_{i=1}^N\sum_{j=1}^P\frac{\lambda_j^{*^2}}{\sigma_j^{*^2}}\frac{1}{2}\bigg[(\sum_{k'=1}^KI_{jk'}^c\alpha_{ik'}^*)^2 + (\sum_{k=1}^Kq_{jk}^c(q_{ik}^{\alpha})^2) + (\sum_{k=1}^Kq_{jk}^c\tvar(\alpha_{ik}))  \\
& \quad - 2(\sum_{k'=1}^KI_{jk'}^c\alpha_{ik'}^{*})(\sum_{k=1}^Kq_{jk}^cq_{ik}^{\alpha})+  (\sum_{k=1}^Kq_{jk}^cq_{ik}^{\alpha})^2 - (\sum_{k=1}^Kq_{jk}^cq_{ik}^{\alpha})^2\bigg] \\
& = \sum_{i=1}^N\sum_{j=1}^P\frac{\lambda_j^{*^2}}{\sigma_j^{*^2}}\frac{1}{2}\bigg[\underbrace{\left((\sum_{k'=1}^KI_{jk'}^c\alpha_{ik'}^*) - (\sum_{k=1}^Kq_{jk}^cq_{ik}^{\alpha})\right)^2}_{\textcolor{blue}{(a)}} + \underbrace{(\sum_{k=1}^Kq_{jk}^c\tvar(\alpha_{ik}))}_{\textcolor{blue}{(b)}} \\
& \quad +\underbrace{(\sum_{k=1}^Kq_{jk}^c(q_{ik}^{\alpha})^2) - (\sum_{k=1}^Kq_{jk}^cq_{ik}^{\alpha})^2 }_{\textcolor{blue}{(c)}} \bigg]. \tag{S1} \label{eq.s1}
\end{align*}

Equation (\ref{eq.s1}) is equal to zero if and only if the three components (a), (b) and (c) are equal to zero respectively, which is equivalent to the followings conditions (C-1) to (C-3).
\begin{itemize}
    \item[(C-1)] $\sum_{k'=1}^KI_{jk'}^c\alpha_{ik'}^* = \sum_{k=1}^Kq_{jk}^cq_{ik}^{\alpha}$, for $1\leq i \leq N, 1 \leq j \leq P$.
    \item[(C-2)] $\sum_{k=1}^Kq_{jk}^c\tvar(\alpha_{ik}) = 0$, for  $1\leq i \leq N, 1 \leq j \leq P$.
    \item[(C-3)]
    $(\sum_{k=1}^Kq_{jk}^c(q_{ik}^{\alpha})^2) - (\sum_{k=1}^Kq_{jk}^cq_{ik}^{\alpha})^2 = 0$, for  $1\leq i \leq N, 1 \leq j \leq P$.
\end{itemize}
 By Jensen's inequality, the equality in (C-3) holds if either row $q_{j\cdot}^c$ has only $\{0,1\}$ as entries with row summation equal to one, or $q_{ik}^{\alpha}$'s have constant values across $k$ at which $q_{jk}^c$ are non-zero for all $i$.

Let $\bic, \balp^*, \bqc, \bqa$ denote the $P\times K$ matrix $[I_{jk}^c]$, $N\times K$ matrix $[\alpha_{ik}^*]$, $P\times K$ matrix $[q_{jk}^c]$ and $N\times K$ matrix $[q_{ik}^{\alpha}]$ respectively. Then (C-1) can be written as $\bic\balp^T = \bqc\boldsymbol{q}^{\alpha T}$, with condition that $\bic\balp^{*T}$ is of full rank $K$, i.e. $\bic, \balp^*$ are of full rank $K$ respectively, which guarantees that three is no missing class and no collinearity among columns of $\balp^*$. Consequently, $\bqc\boldsymbol{q}^{\alpha T}$ is also of full rank $K$ with each component matrix being full rank $K$.

Observing the fact that $\bqa$ is of full rank $K$, we use the proof of contradiction to show that $\bqc$ is a $P\times K$ matrix with only $\{0,1\}$ entries, with each row summing to one.

Suppose for the row $j$ of $\bqc$, there are two non-zero entries, i.e. $q_{jk}^c\neq 0, q_{jk'}^c\neq 0 (k\neq k')$. Then by condition (C-3),  $q_{ik}^{\alpha} = q_{ik'}^{\alpha}$ for all $i$,  which implies that there are duplicate columns in $\bqa$, contradicting to the statement  that $\bqa$ is of full rank $K$. Therefore $\bqc$ is a $P\times K$ matrix with only $\{0,1\}$ entries and each row sums to one. It's straightforward to show that $\bqc = \bic $ and $\bqa = \balp^*$ is the solution to equation (\ref{eq.s1}) equal to zero. 

In the last step, we prove that the solution is unique up to the permutation of labels. 

Let $\alpha_{\cdot k}^*, q_{\cdot k}^{\alpha}$ denote the column $k$ of the corresponding matrix. Then the $j$-th row of matrix $\bic \balp^{*T}$ is
\begin{align*}
    [\bic \balp^{*T}]_{j\cdot} & = I^c_{j1}(\alpha_{\cdot 1}^*)^T + ...+I^c_{jK}(\alpha_{\cdot K}^*)^T
\end{align*}
together with the condition that $1 = \sum_{k=1}^KI_{jk}^c$, it
implies that the $j$-th row of matrix $\bic \balp^{*T}$ is the $k$-th column of $\balp^*$ where $I_{jk}^c = 1$. Therefore, the rows of $\bic \balp^{*T}$ is made of the columns of $\balp^*$. The number of times that the $k$-th column of $\balp^*$ appearing in the rows of $\bic \balp^{*T}$ depends on the number of objects that belong to the cluster $k$. Similarly, since $\bqc$ only has $\{0,1\}$ entries and each row sums to one, the rows of $\bqc\boldsymbol{q}^{\alpha T}$ consist of columns of $\bqa$. Consequently, condition  $\bic\balp^T = \bqc\boldsymbol{q}^{\alpha T}$ holds if and only if that after a column permutation $\V{P}_{K\times K}$, $\bqa\V{P} = \balp^*$ and  $\bqc\V{P} = \bic$. Therefore, $\bqc = \bic $ and $\bqa = \balp^*$ is the unique solution up to the permutation of labels. 
\end{proof}

%%%%%%%%%%%%%%%%%%%%%%%%%%%%%%%%%%%%%%%%%%%%%%%%%%%%%%%%%%%%%%%%%%%%%%%%%%%%%%

\subsubsection*{A3 Proof of Proposition 2}

\begin{proposition*}
Define the distance $d(\bic, \bqc)$ between $\bic, \bqc$ as
\begin{align*}
    d(\bic, \bqc) & = 1-\tr[\mathbb{R}(\bic, \bqc)],
\end{align*}
where $\mathbb{R}(\bic, \bqc)$ is a $K\times K$ confusion matrix defined by
\begin{align*}
\mathbb{R}_{kk'}(\bic, \bqc) & = \frac{1}{P}\sum_{j=1}^PI_{jk}^cq_{jk'}^c.
\end{align*}

The distance $d(\bic, \bqc)$ is equivalent to the distance between $\bic, \bqc$ in $L_1$ norm, provided
that at least one of them consists of only $\{0,1\}$ values.
\end{proposition*}

\begin{proof}
Since $d(\V{I}^c, \bqc)$ is defined as 
\begin{align*}
   d(\V{I}^c, \bqc) & = 1- \tr[\mathbb{R}(\bic, \bqc)] = 1- \frac{1}{P}\sum_{j=1}^P\sum_{k=1}^KI_{jk}^cq_{jk}^c,
\end{align*}
the distance can be written as either
\begin{align*}
  d(\V{I}^c, \bqc)  & = \frac{1}{P}\sum_{j=1}^P\sum_{k=1}^KI_{jk}^c(1-q_{jk}^c) = \frac{1}{P}\sum_{j=1}^P\sum_{k=1}^K I(c_j=k)|I_{jk}^c - q_{jk}^c|,
\end{align*}
or
\begin{align*}
     d(\V{I}^c, \bqc)  & = \frac{1}{P}\sum_{j=1}^P\sum_{k=1}^K(1-I_{jk}^c)q_{jk}^c = \frac{1}{P}\sum_{j=1}^P\sum_{k=1}^K I(c_j\neq k)|I_{jk}^c - q_{jk}^c|.
\end{align*}
Therefore,
\begin{align*}
    d(\V{I}^c, \bqc) & = \frac{1}{2P}\sum_{j=1}^P\sum_{k=1}^K|I_{jk}^c - q_{jk}^c| = \frac{1}{2P}\norm{\bic-\bqc}_1.
\end{align*}

\end{proof}

%%%%%%%%%%%%%%%%%%%%%%%%%%%%%%%%%%%%%%%%%%%%%%%%%%%%%%%%%%%%%%%%%%%%%%%%%%%%%%

\subsubsection*{A4 Proof of Proposition 3}

\begin{proposition*}
 Assume that for a positive constant $\gamma_1$, $\min_j\left\{\frac{1}{2}\frac{\lambda_j^{*^2}}{\sigma_j^{*^2}}\right\}>\gamma_1>0$ and $m = \min_{1\leq k < l \leq K}(\omega_{kk}^*+\omega_{ll}^*-2\omega_{kl}^*)>0$. Then as $N,P\longrightarrow \infty$, for any $\bqc$ and $\bqa$,
\begin{align*}
& \mathbb{P}\left(\bar{J}(\bic, \balp^*) -  \bar{J}(\bqc, \bqa) \geq \frac{PNm\gamma_1}{16} \frac{1}{P}\norm{\bic-\bqc}_1\right) \longrightarrow 1.
\end{align*}
\end{proposition*}

\begin{proof}

From equation \ref{eq.s1} we have
\begin{align*}
   & \bar{J}(\bic, \balp^*; \Phi^*) -  \bar{J}(\bqc, \bqa; \Phi^*)\\
    & =
    \sum_{i=1}^N\sum_{j=1}^P\frac{\lambda_j^{*^2}}{\sigma_j^{*^2}}\frac{1}{2}\bigg[\left((\sum_{k'=1}^KI_{jk'}^c\alpha_{ik'}^*) - (\sum_{k=1}^Kq_{jk}^cq_{ik}^{\alpha})\right)^2 \\
    & \quad + (\sum_{k=1}^Kq_{jk}^c\tvar(\alpha_{ik})) +(\sum_{k=1}^Kq_{jk}^c(q_{ik}^{\alpha})^2) - (\sum_{k=1}^Kq_{jk}^cq_{ik}^{\alpha})^2  \bigg] \\
& \geq \min_j\left\{\frac{1}{2}\frac{\lambda_j^{*^2}}{\sigma_j^{*^2}}\right\}\sum_{i=1}^N\sum_{j=1}^P\bigg[\left((\sum_{k'=1}^KI_{jk'}^c\alpha_{ik'}^*) - (\sum_{k=1}^Kq_{jk}^cq_{ik}^{\alpha})\right)^2 +(\sum_{k=1}^Kq_{jk}^c(q_{ik}^{\alpha})^2) - (\sum_{k=1}^Kq_{jk}^cq_{ik}^{\alpha})^2  \bigg]  \\
& =  \gamma_1\sum_{i=1}^N\sum_{l=1}^K\sum_{j\in C_l}\bigg[\left(\alpha_{il}^* - \sum_{k=1}^Kq_{jk}^cq_{ik}^{\alpha}\right)^2 +(\sum_{k=1}^Kq_{jk}^c(q_{ik}^{\alpha})^2) - (\sum_{k=1}^Kq_{jk}^cq_{ik}^{\alpha})^2  \bigg]\\
& = \gamma_1\sum_{i=1}^N\sum_{l=1}^K\sum_{j\in C_l}\bigg[\sum_{k=1}^Kq_{jk}^c\left(\alpha_{il}^* - q_{ik}^{\alpha}\right)^2 \bigg]\\
& = \gamma_1\sum_{l=1}^K\sum_{j\in C_l}\sum_{k=1}^Kq_{jk}^c\norm{\alpha_{\cdot l}^* - q_{\cdot k}^{\alpha}}_2^2,
\tag{S2}\label{eq.s2}
\end{align*}
where $\gamma_1 = \min_j\left\{\frac{1}{2}\frac{\lambda_j^2}{\sigma_j^2}\right\} $, $\alpha_{\cdot l}^*$ and $q_{\cdot k}^{\alpha}$ are the column $l$ and $k$ of $\balp^*$ and $\bqa$ respectively. The second to the last step is based on the mean square error(MSE) equation
\begin{align*}
 \mathbb{E}\left(\theta -\hat{\theta}\right)^2 = \left(\mathbb{E}\hat{\theta} - \theta\right)^2 + \mathbb{E}\left(\hat{\theta} - \mathbb{E}\hat{\theta}\right)^2. 
\end{align*}

Let $\gamma_2 =  \min_{k\neq l}\norm{\alpha_{\cdot k}^*-\alpha_{\cdot l}^*}_2^2$. Since $\balp^*$ is of full rank $K$, $\gamma_2 > 0$. Then we can tighten the lower bound of equation (\ref{eq.s2}) as follows. 

\begin{align*}
  & \gamma_1\sum_{l=1}^K\sum_{j\in C_l}\sum_{k=1}^Kq_{jk}^c\norm{\alpha_{\cdot l}^* - q_{\cdot k}^{\alpha}}_2^2 \\
  & = \gamma_1\sum_{j=1}^P\sum_{k=1}^Kq_{jk}^c\norm{\alpha_{\cdot c_j}^* - q_{\cdot k}^{\alpha}}_2^2 \geq \gamma_1\sum_{j=1}^P\sum_{k\neq c_j}^Kq_{jk}^c\norm{\alpha_{\cdot c_j}^* - q_{\cdot k}^{\alpha}}_2^2
 \geq \gamma_1 \sum_{j=1}^P\sum_{k\neq c_j}^Kq_{jk}^{c}\frac{\gamma_2}{4} \\
 & =\frac{\gamma_1\gamma_2}{4}\sum_{j=1}^P\sum_{k=1}^K(1-I_{jk}^c)q_{jk}^c\\
 & = \frac{\gamma_1\gamma_2}{4}\Big[P - P\frac{1}{P}\sum_{j=1}^P\sum_{k=1}^KI_{jk}^cq_{jk}^c\Big]= \frac{\gamma_1\gamma_2P}{4}\Big[1 - \tr(\mathbb{R}(\bic, \bqc))\Big]= \frac{\gamma_1\gamma_2P}{4}d(\bic, \bqc)\\
 & =\frac{P\gamma_1\gamma_2}{4}\frac{1}{2P}\norm{\V{I}^c - \bqc}_1.
 \tag{S3} \label{eq.s3}
\end{align*}

Next we prove that not only $\gamma_2 >0$, it also has the same order as $N$. According to the model assumption that $\balp_i^*\sim N(\bf{0}, \bome^*)$, we have
\begin{align*}
   & \alpha_{ik}^* -\alpha_{il}^*\sim N(0, \omega_{kk}^*+\omega_{ll}^*-2\omega_{kl}^*)\\
   & \sum_{i=1}^N(\alpha_{ik}^* -\alpha_{il}^*)^2 \sim  (\omega_{kk}^*+\omega_{ll}^*-2\omega_{kl}^*)\chi_N^2,
\end{align*}
where $\chi_N^2$ is a chi-squared distribution with $N$ degrees of freedom. Let $A_{kl} = \sum_{i=1}^N(\alpha_{ik}^* -\alpha_{il}^*)^2$ and $m = \min_{1\leq k < l \leq K}(\omega_{kk}^*+\omega_{ll}^*-2\omega_{kl}^*)$. By the sub-exponential tail bounds of chi-squared random variable,
\begin{align*}
    & \mathbb{P}\left(A_{kl} < \frac{Nm}{2}\right)\\
    & \leq
    \mathbb{P}\left(A_{kl} \leq \frac{N(\omega_{kk}^*+\omega_{ll}^*-2\omega_{kl}^*)}{2}\right)\\
    & \leq \exp{-\frac{N}{16}}.
\end{align*}
Then
\begin{align*}
   & \mathbb{P}\left(\gamma_2 > \frac{Nm}{2}\right) =  \mathbb{P}\left(\min_{1\leq k<l\leq K}A_{kl} > \frac{Nm}{2}\right)\\
   & = 1- \mathbb{P}\left(\exists k,l; A_{kl} < \frac{Nm}{2}\right)\\
   & \geq 1- \bigcup_{1\leq k<l\leq K}\mathbb{P}\left(A_{kl} < \frac{Nm}{2}\right)\\
   & \geq 1- \bigcup_{1\leq k<l\leq K}\exp{-\frac{N}{16}}\\
   & \geq 1- \frac{K(K-1)}{2}\exp{-\frac{N}{16}},
\end{align*}
which implies that $\gamma_2$ is of the same order as $Nm/2$. Therefore as $N,P\longrightarrow \infty$, 
\begin{align*}
  \mathbb{P}\left(\bar{J}(\bic, \balp^*; \Phi^*) -  \bar{J}(\bqc, \bqa; \Phi^*) \geq \frac{PNm\gamma_1}{16} \frac{1}{P}\norm{\bic-\bqc}_1\right) \longrightarrow 1.  
\end{align*}

\end{proof}
%%%%%%%%%%%%%%%%%%%%%%%%%%%%%%%%%%%%%%%%%%%%%%%%%%%%%%%%%%%%%%%%%%%%%%%%%%%%%%

\subsubsection*{A5 Proof of Proposition 4}

\begin{proposition*}
 Assume that $X_{ij}'s$ are centered. Let $\hat{\lambda}_j = \sum_{t=1}^P\frac{\sum_{i=1}^NX_{ij}X_{it}}{PN}$ and $\lambda_j^* = \sum_{t=1}^P \frac{\lambda_j\lambda_t\omega_{c_jc_t}}{P}$ as in the canonical form. As $N,P\rightarrow \infty$ with $\log(P)/N = o(1)$ and $\max_j\{\sigma_j^{*2}\}=o(P)$,
\begin{align*}
   & \mathbb{P}(|\hat{\lambda}_j - \lambda_j^*|\geq \epsilon | c^*) \longrightarrow 0.
\end{align*}
\end{proposition*}

\begin{proof}

Given the model assumption that $\text{Cov}(X_{j}, X_{j'}|\V{c}) = \lambda_j\lambda_{j'}\omega_{c_j c_{j'}} +  \sigma_j^2I(j=j')$, we have
\begin{align*}
 &   \mathbb{P}(|\hat{\lambda}_j - \lambda_j^*|\geq \epsilon| \V{c}^*)\\
 = & \mathbb{P}(|\hat{\lambda}_j - \mathbb{E}(\hat{\lambda}_j) + \mathbb{E}(\hat{\lambda}_j) - \lambda_j^*|\geq \epsilon| \V{c}^*)\\
 \leq & \mathbb{P}(|\hat{\lambda}_j - \mathbb{E}(\hat{\lambda}_j)|\geq \epsilon/2| \V{c}^*) + \mathbb{P}(| \mathbb{E}(\hat{\lambda}_j) - \lambda_j^*|\geq \epsilon/2|\V{c}^*)\\
 = & \mathbb{P}\left(\left|\sum_{t=1}^P\frac{\sum_{i=1}^NX_{ij}X_{it}}{PN} - \sum_{t=1}^P \frac{\lambda_j\lambda_t\omega_{c_jc_t}}{P} - \frac{\sigma_j^{*2}}{P}\right|\geq \epsilon/2| \V{c}^*\right) + \mathbb{P}\left(\left| \frac{\sigma_j^{*2}}{P}\right|\geq \epsilon/2| \V{c}^*\right)\\
 \leq & \sum_{t=1}^P\mathbb{P}\left(\left|\frac{\sum_{i=1}^NX_{ij}X_{it}}{N} - \lambda_j\lambda_t\omega_{c_jc_t} - \sigma_j^{*2}\right|\geq \epsilon/2| \V{c}^*\right) + o(1) \\
 \leq & PC_1\exp(-C_2N\epsilon^2) + o(1),
 \end{align*}
where $C_1 = \max_{t}{C_{t1}}, C_2 = \min_{t}{C_{t2}}$.
The second to last inequality is due to the tail bound of the product of two sub-gaussians being sub-exponential.
\end{proof}

%%%%%%%%%%%%%%%%%%%%%%%%%%%%%%%%%%%%%%%%%%%%%%%%%%%%%%%%%%%%%%%%%%%%%%%%%%%%%%

\subsubsection*{A6 Proof of Theorem 1}

\begin{theorem*}
For all $ \epsilon > 0$, as $N, P \rightarrow \infty$ and $\log(P)/N = o(1)$,
\begin{align*}
    \mathbb{P}\left(\underset{q_1\in C_c, q_2 \in C_{\alpha}}{\max}\left|\hat{J}(\bqc, \bqa; \hat{\Phi}) - \bar{J}(\bqc, \bqa; \Phi^*)\right|\geq NP\epsilon  \middle| \V{c}^* \right) \longrightarrow 0,
\end{align*}
where $C_c = \{\bqc: \bqc \in \mathbb{R}^{P\times K}, q_{jk}^c \in [0,1], \sum_{k=1}^Kq_{jk}^c = 1\}$ and $C_{\alpha} = \{\bqa: \bqa \in \mathbb{R}^{N\times K}, q_{ik}^{\alpha} \in [-B_1,B_1], \bqas_{ik} \in [0, B_2]\}$ are the compact domain for the corresponding parameters. $\lambda_j^*$ has upper bound such that $\max_j|\lambda_j^*| < B_3/3$ and $\min_j\left\{\frac{1}{2}\frac{\lambda_j^{*^2}}{\sigma_j^{*^2}}\right\}>\gamma_1>0$, where $B_1, B_2, B_3, \gamma_1$ are  positive constants. 
\end{theorem*}

\begin{proof}

Write
\begin{align*}
\hat{J}_1(\bqc, \bqa; \hat{\Phi}) & = \sum_{i=1}^N\sum_{j=1}^P\left(-\frac{X_{ij}^2}{2\hat{\sigma}_j^2}\right)\\ 
\bar{J}_1(\bqc, \bqa; \Phi^*) & = \sum_{i=1}^N\sum_{j=1}^P\left(-\frac{\mathbb{E}(X_{ij}^2|\balp^*,\V{c}^*)}{2\sigma_j^{*2}}\right)\\ 
\hat{J}_2(\bqc, \bqa; \hat{\Phi}) & = \sum_{i=1}^N\sum_{j=1}^P\sum_{k=1}^K\left(-\frac{\hat{\lambda}_j^2q_{jk}^c\mathbb{E}_{q_2}(\alpha_{ik}^2)}{2\hat{\sigma}_j^2}\right) \\
\bar{J}_2(\bqc, \bqa; \Phi^*) & = \sum_{i=1}^N\sum_{j=1}^P\sum_{k=1}^K\left(-\frac{\lambda_j^{*2}q_{jk}^c\mathbb{E}_{q_2}(\alpha_{ik}^2)}{2\sigma_j^{*2}}\right) \\ 
\hat{J}_3(\bqc, \bqa; \hat{\Phi}) & = \sum_{i=1}^N\sum_{j=1}^P\sum_{k=1}^K\left(\frac{q_{jk}^c\hat{\lambda}_jX_{ij}\mathbb{E}_{q_2}(\alpha_{ik})}{\hat{\sigma}_j^2}\right)\\
\bar{J}_3(\bqc, \bqa; \Phi^*) & = \sum_{i=1}^N\sum_{j=1}^P\sum_{k=1}^K\left(\frac{q_{jk}^c{\lambda}_j^*\mathbb{E}(X_{ij}|\balp^*,\V{c}^*)\mathbb{E}_{q_2}(\alpha_{ik})}{\sigma_j^{*2}}\right)\\ 
\hat{J}_4(\bqc, \bqa; \hat{\Phi}) & = \sum_{j=1}^P\left(\sum_{k=1}^Kq_{jk}^c\ln\hat{\pi}_k\right) + \sum_{i=1}^N\left(-\frac{1}{2}\ln|\hat{\bome}| - \frac{1}{2}\tr{(\mathbb{E}_{q_2}(\alpha_i\alpha_i^T)\hat{\bome}^{-1})}\right)\\
& + \sum_{i=1}^N\sum_{j=1}^P\left(-\frac{1}{2}\ln\hat{\sigma}_j^2\right) + \sum_{j=1}^P\sum_{k=1}^Kq_{jk}^c\ln q_{jk}^c + \sum_{i=1}^N\left(-\frac{K}{2}\ln2\pi -\frac{1}{2}\ln|\M{V}|\right)\\
& -\frac{NK}{2}.
\end{align*}
It's straightforward to check that 
\begin{align*}
  \hat{J}(\bqc, \bqa; \hat{\Phi}) & = \hat{J}_1(\bqc, \bqa; \hat{\Phi}) + \hat{J}_2(\bqc, \bqa; \hat{\Phi})+ \hat{J}_3(\bqc, \bqa; \hat{\Phi})+ \hat{J}_4(\bqc, \bqa; \hat{\Phi})  \\
  \bar{J}(\bqc, \bqa; \Phi^*) & = \bar{J}_1(\bqc, \bqa; \Phi^*)+\bar{J}_2(\bqc, \bqa; \Phi^*) + \bar{J}_3(\bqc, \bqa; \Phi^*).
\end{align*}

We prove the uniform convergence of $\hat{J}(\cdot)$ to $\bar{J}(\cdot)$ by showing that the components $\hat{J}_1(\cdot)$, $\hat{J}_2(\cdot)$, $\hat{J}_3(\cdot)$ uniformly converge to their population counterparts respectively. The last term $\hat{J}_4(\cdot)$ is omitted because it's of smaller order and diminishes asymptotically. Note that $\vsigHat$ and $\vsigStar$ do not contribute to the uniform convergence and therefore are ignored in the proof.

We first prove that for all $\epsilon > 0$, as $N, P \rightarrow \infty$,
\begin{align*}
    \mathbb{P}\left(\underset{q_1\in C_c, q_2 \in C_{\alpha}}{\max}\left|\hat{J}_1(\bqc, \bqa; \hat{\Phi}) - \bar{J}_1(\bqc, \bqa; \Phi^*)\right|\geq NP\epsilon |\V{c}^* \right) \rightarrow 0.
\end{align*}

Write
\begin{align*}
    &\left|\hat{J}_1(\bqc, \bqa; \hat{\Phi}) - \bar{J}_1(\bqc, \bqa; \Phi^*)\right| \\
    & = \left|\sum_{i=1}^N\sum_{j=1}^P\left(\frac{X_{ij}^2}{2\hat{\sigma}_j^2} - \frac{\mathbb{E}(X_{ij}^2|\V{\alpha}^*, \V{c}^*)}{2\sigma_j^{*2}}\right)\right|\\
    & \sim \left|\sum_{i=1}^N\sum_{j=1}^P\left(X_{ij}^2 - \mathbb{E}(X_{ij}^2|\V{\alpha}^*, \V{c}^*)\right)\right|,
\end{align*}
then by the tail bound inequality of exponential distributions, we have
\begin{align*}
    &\mathbb{P}\left(\underset{q_1\in C_c, q_2 \in C_{\alpha}}{\max}\left|\hat{J}_1(\bqc, \bqa; \hat{\Phi}) - \bar{J}_1(\bqc, \bqa; \Phi^*)\right|\geq NP\epsilon |\V{c}^* \right) \\
    = & \mathbb{P}\left(\underset{q_1\in C_c, q_2 \in C_{\alpha}}{\max}\left|\sum_{i=1}^N\sum_{j=1}^P(X_{ij}^2-\mathbb{E}(X_{ij}^2|\V{\alpha}^*,  \V{c}^*))\right|\geq NP\epsilon |\V{c}^* \right)\\
    \leq & 2\exp\left(-\frac{NP^2\epsilon^2}{ 64\sum_{j=1}^P\sigma_j^{*^4}}\right).
\end{align*}

Next we prove that for all $\epsilon > 0$, as $N, P \rightarrow \infty$ and $\ln(P)/N = o(1)$,
\begin{align*}
    \mathbb{P}\left(\underset{q_1\in C_c, q_2 \in C_{\alpha}}{\max}\left|\hat{J}_2(\bqc, \bqa; \hat{\Phi}) - \bar{J}_2(\bqc, \bqa; \Phi^*)\right|\geq NP\epsilon |\V{c}^* \right) \rightarrow 0.
\end{align*}

Write 
\begin{align*}
    &\left|\hat{J}_2(\bqc, \bqa; \hat{\Phi}) - \bar{J}_2(\bqc, \bqa; \Phi^*)\right| \\
    & = \left|\sum_{i=1}^N\sum_{j=1}^P\sum_{k=1}^K\left(-\frac{\hat{\lambda}_j^2q_{jk}^c\mathbb{E}_{q_2}(\alpha_{ik}^2)}{2\hat{\sigma}_j^2}+\frac{\lambda_j^{*2}q_{jk}^c\mathbb{E}_{q_2}(\alpha_{ik}^2)}{2\sigma_j^{*2}}\right)\right|\\
    & \sim \left|\sum_{i=1}^N\sum_{j=1}^P\sum_{k=1}^K\left(\hat{\lambda}_j^2q_{jk}^c\mathbb{E}_{q_2}(\alpha_{ik}^2) -\lambda_j^{*2}q_{jk}^c\mathbb{E}_{q_2}(\alpha_{ik}^2)\right)\right|\\
    & = \left|\sum_{i=1}^N\sum_{j=1}^P\sum_{k=1}^K q_{jk}^c\mathbb{E}_{q_2}(\alpha_{ik}^2)\left(\hat{\lambda}_j^2 -\lambda_j^{*2}\right)\right|\\
    & \leq \sum_{i=1}^N\sum_{k=1}^K\sum_{j=1}^P\left|q_{jk}^c\mathbb{E}_{q_2}(\alpha_{ik}^2)\right|\left|\hat{\lambda}_j^2 -\lambda_j^{*2}\right|\\
    & \leq NKB_2\sum_{j=1}^P\left|\hat{\lambda}_j^2 -\lambda_j^{*2}\right| \\
    & = NKB_2\sum_{j=1}^P\left|\hat{\lambda}_j -\lambda_j^{*}\right|\left|\hat{\lambda}_j +\lambda_j^{*}\right|
\end{align*}

Then 
\begin{align*}
&  \mathbb{P}\left(\underset{q_1\in C_c, q_2 \in C_{\alpha}}{\max}\left|\hat{J}_2(\bqc, \bqa; \hat{\Phi}) - \bar{J}_2(\bqc, \bqa; \Phi^*)\right|\geq NP\epsilon |\V{c}^* \right) \\
& \leq \mathbb{P}\left(NKB_2\sum_{j=1}^P\left|\hat{\lambda}_j -\lambda_j^{*}\right|\left|\hat{\lambda}_j +\lambda_j^{*}\right|\geq NP\epsilon |\V{c}^* \right) \\
& \leq \mathbb{P}\left(NKB_2\sum_{j=1}^P\left|\hat{\lambda}_j -\lambda_j^{*}\right|\left|\hat{\lambda}_j +\lambda_j^{*}\right|\geq NP\epsilon; \exists j, \left|\hat{\lambda}_j -\lambda_j^{*}\right| \geq \epsilon |\V{c}^* \right) \\
& \quad + \mathbb{P}\left(NKB_2\sum_{j=1}^P\left|\hat{\lambda}_j -\lambda_j^{*}\right|\left|\hat{\lambda}_j +\lambda_j^{*}\right|\geq NP\epsilon; \forall j, \left|\hat{\lambda}_j -\lambda_j^{*}\right| < \epsilon |\V{c}^* \right) \\
& \leq \sum_{j=1}^P\mathbb{P}\left( \left|\hat{\lambda}_j -\lambda_j^{*}\right| \geq \epsilon |\V{c}^* \right)  + \mathbb{P}\left(NKB_2\sum_{j=1}^P\left|\hat{\lambda}_j -\lambda_j^{*}\right|\left| 2\lambda_j^{*} + \epsilon\right|\geq NP\epsilon |\V{c}^* \right)\\
& \leq \sum_{j=1}^P\mathbb{P}\left( \left|\hat{\lambda}_j -\lambda_j^{*}\right| \geq \epsilon |\V{c}^* \right)  + \mathbb{P}\left(NKB_2B_3\sum_{j=1}^P\left|\hat{\lambda}_j -\lambda_j^{*}\right|\geq NP\epsilon |\V{c}^* \right)\\
& \leq \sum_{j=1}^P\mathbb{P}\left( \left|\hat{\lambda}_j -\lambda_j^{*}\right| \geq \epsilon |\V{c}^* \right)  + \sum_{j=1}^P \mathbb{P}\left(NKB_2B_3\left|\hat{\lambda}_j -\lambda_j^{*}\right|\geq N\epsilon |\V{c}^* \right) \\
& \leq P^2C_1\exp(-C_2N\epsilon^2) +  P^2C_1\exp(-C_2\frac{N\epsilon^2}{K^2B_2^2B_3^2})\\
&\leq P^2C_1\exp(-C_2N\epsilon^2).
\end{align*}
The second to last inequality is the result of using the proposition 4.

Lastly we prove that for all $\epsilon > 0$, as $N, P \rightarrow \infty$ and $\ln(P)/N = o(1)$,
\begin{align*}
    \mathbb{P}\left(\underset{q_1\in C_c, q_2 \in C_{\alpha}}{\max}\left|\hat{J}_3(\bqc, \bqa; \hat{\Phi}) - \bar{J}_3(\bqc, \bqa; \Phi^*)\right|\geq NP\epsilon |\V{c}^* \right) \rightarrow 0.
\end{align*}

Write
\begin{align*}
    &\quad \left|\hat{J}_3(\bqc, \bqa) - \bar{J}_3(\bqc, \bqa)\right| \\
    & = \left| \sum_{i=1}^N\sum_{j=1}^P\sum_{k=1}^K\left(\frac{\hat{\lambda}_jq_{jk}^cq_{ik}^{\alpha}X_{ij}}{\hat{\sigma}_j^2}-\frac{\lambda_j^{*}q_{jk}^cq_{ik}^{\alpha}\mathbb{E}(X_{ij}|\balp^*,\V{c}^*)}{\sigma_j^{*2}}\right) \right|\\
    & \sim \left| \sum_{i=1}^N\sum_{j=1}^P\sum_{k=1}^K\left(\hat{\lambda}_jq_{jk}^cq_{ik}^{\alpha}X_{ij}-\lambda_j^{*}q_{jk}^cq_{ik}^{\alpha}\mathbb{E}(X_{ij}|\balp^*,\V{c}^*)\right) \right| \\
    & \leq \sum_{k=1}^K \left| \sum_{i=1}^N\sum_{j=1}^P\left(\hat{\lambda}_jX_{ij} -\lambda_j^{*}\mathbb{E}(X_{ij}|\balp^*,\V{c}^*) \right)q_{jk}^cq_{ik}^{\alpha} \right|\\
    & = \sum_{k=1}^K \bigg| \sum_{i=1}^N\sum_{j=1}^P\bigg(\lambda_j^*(X_{ij} - \mathbb{E}(X_{ij}|\balp^*,\V{c}^*)) +(\hat{\lambda}_j-\lambda_j^*)(X_{ij} - \mathbb{E}(X_{ij}|\balp^*,\V{c}^*)) \\
    & \quad + (\hat{\lambda}_j-\lambda_j^*) \mathbb{E}(X_{ij}|\balp^*,\V{c}^*) \bigg)q_{jk}^cq_{ik}^{\alpha} \bigg|\\
    & \leq \underbrace{\sum_{k=1}^K \left| \sum_{i=1}^N\sum_{j=1}^P\left(\lambda_j^*(X_{ij} - \mathbb{E}(X_{ij}|\balp^*,\V{c}^*))\right)q_{jk}^cq_{ik}^{\alpha} \right|}_{(a)} +\\
    & \quad \underbrace{\sum_{k=1}^K \left| \sum_{i=1}^N\sum_{j=1}^P\left((\hat{\lambda}_j-\lambda_j^*)(X_{ij} - \mathbb{E}(X_{ij}|\balp^*,\V{c}^*))\right)q_{jk}^cq_{ik}^{\alpha} \right|}_{(b)} + \\
    & \quad \underbrace{\sum_{k=1}^K \left| \sum_{i=1}^N\sum_{j=1}^P\left((\hat{\lambda}_j-\lambda_j^*) \mathbb{E}(X_{ij}|\balp^*,\V{c}^*) \right)q_{jk}^cq_{ik}^{\alpha} \right|}_{(c)}.
\end{align*}

We first prove the following statement that

\begin{align*}
 & \underset{q_1\in C_c, q_2 \in C_{\alpha}}{\max} \left| \sum_{i=1}^N\sum_{j=1}^P\left(X_{ij} -\mathbb{E}(X_{ij}|\balp^*,\V{c}^*) \right)q_{jk}^cq_{ik}^{\alpha}  \right|\\
   & = \underset{q_1\in \{0,1\}, q_2 \in \{-B_1, B_1\}}{\max} \left| \sum_{i=1}^N\sum_{j=1}^P\left(X_{ij} -\mathbb{E}(X_{ij}|\balp^*,\V{c}^*) \right)q_{jk}^cq_{ik}^{\alpha} \right|.
\end{align*}
Let $f(\mathbf{u},\mathbf{v}) = \sum_{i=1}^n\sum_{j=1}^p(X_{ij}- \mu_{ij})u_iv_j$, where $\mu_{ij}=\mathbb{E}(X_{ij}|\balp^*,\V{c}^*), u_i\in [0,1], v_j \in [-B_1, B_1]$. If the maximum occurs at $(\bf{u},\bf{v})$ with $v_1\in(-B_1, B_1)$, consider $\mathbf{v}^{'},\mathbf{v}^{''}$ with $v_1^{'}=-B_1,v_1^{''}=B_1$ and the other entries are identical to that of $\mathbf{v}$. Then we can write $f(\mathbf{u},\mathbf{v}) =\frac{B_1-v_1}{2B_1}f(\mathbf{u},\mathbf{v}^{'})+\frac{v_1+B_1}{2B_1}f(\mathbf{u},\mathbf{v}^{''})$. Since $f(\mathbf{u},\mathbf{v})$ is a linear function of $v_1$, the value of $f(\mathbf{u},\mathbf{v})$ is between $f(\mathbf{u},\mathbf{v}^{'})$ and $f(\mathbf{u},\mathbf{v}^{''})$, which implies that both $(\mathbf{u},\mathbf{v}^{'})$ and $(\mathbf{u},\mathbf{v}^{''})$ are maximizers and we take either $(\mathbf{u},\mathbf{v}^{'})$ or $(\mathbf{u},\mathbf{v}^{''})$ instead of $(\mathbf{u},\mathbf{v})$. If there are other entries of $\mathbf{v}$ strictly between $(-B_1,B_1)$, we can use the same argument until we find a maximizer with all entries equal to $-B_1$ or $B_1$. The same argument applies to $\mathbf{u}$ being an maximizer with all entries equal to 0 or 1. Next we provide the upper bounds of the three components (a), (b) and (c).

The first term (a) satisfies the inequality that
\begin{align*}
    & \mathbb{P}\left(\underset{q_1\in C_c, q_2 \in C_{\alpha}}{\max}
    \sum_{k=1}^K \left| \sum_{i=1}^N\sum_{j=1}^P\left(\lambda_j^*X_{ij} -\lambda_j^*\mathbb{E}(X_{ij}|\balp^*,\V{c}^*) \right)q_{jk}^cq_{ik}^{\alpha}  \right|\geq NP\epsilon |\V{c}^* \right)\\
    =& \mathbb{P}\left(\underset{q_1\in \{0,1\}, q_2 \in \{-B_1, B_1\}}{\max} 
    \sum_{k=1}^K \left| \sum_{i=1}^N\sum_{j=1}^P\left(\lambda_j^*X_{ij} -\lambda_j^*\mathbb{E}(X_{ij}|\balp^*,\V{c}^*) \right)q_{jk}^cq_{ik}^{\alpha}  \right|\geq NP\epsilon |\V{c}^* \right)\\
    \leq & \sum_{k=1}^K\mathbb{P}\left(\underset{q_1\in \{0,1\}, q_2 \in \{-B_1, B_1\}}{\max} 
    \left| \sum_{i=1}^N\sum_{j=1}^P\left(\lambda_j^*X_{ij} -\lambda_j^*\mathbb{E}(X_{ij}|\balp^*,\V{c}^*) \right)q_{jk}^cq_{ik}^{\alpha} \right|\geq NP\frac{\epsilon}{K} |\V{c}^* \right)\\
    \leq & K2^{N+P} 2\exp(-\frac{NP^2\epsilon^2}{2(B_1K)^2\sum_{j=1}^P\lambda_j^{*2}\sigma_j^{*2}}).
\end{align*}

The second term (b) satisfies the inequality that
{\small
\begin{align*}
     & \mathbb{P}\left(\underset{q_1\in C_c, q_2 \in C_{\alpha}}{\max}
    \sum_{k=1}^K \left| \sum_{i=1}^N\sum_{j=1}^P\left((\hat{\lambda}_j-\lambda_j^*)(X_{ij} - \mathbb{E}(X_{ij}|\balp^*,\V{c}^*))\right)q_{jk}^cq_{ik}^{\alpha} \right|
  \geq NP\epsilon |\V{c}^* \right)\\   
  & = \mathbb{P}\bigg(\underset{q_1\in C_c, q_2 \in C_{\alpha}}{\max}
    \sum_{k=1}^K \left| \sum_{i=1}^N\sum_{j=1}^P\left((\hat{\lambda}_j-\lambda_j^*)(X_{ij} - \mathbb{E}(X_{ij}|\balp^*,\V{c}^*))\right)q_{jk}^cq_{ik}^{\alpha} \right|
  \geq NP\epsilon, \\
  & \qquad \qquad \exists j, \left|\hat{\lambda}_j -\lambda_j^{*}\right| \geq \epsilon_1 |\V{c}^* \bigg) \\
  & \quad + \mathbb{P}\bigg(\underset{q_1\in C_c, q_2 \in C_{\alpha}}{\max}
    \sum_{k=1}^K \left| \sum_{i=1}^N\sum_{j=1}^P\left((\hat{\lambda}_j-\lambda_j^*)(X_{ij} - \mathbb{E}(X_{ij}|\balp^*,\V{c}^*))\right)q_{jk}^cq_{ik}^{\alpha} \right|
  \geq NP\epsilon, \\
  & \qquad \qquad  \forall j, \left|\hat{\lambda}_j -\lambda_j^{*}\right| < \epsilon_1 |\V{c}^* \bigg)\\
  & \leq \sum_{j=1}^P\mathbb{P}\left( \left|\hat{\lambda}_j -\lambda_j^{*}\right| \geq \epsilon_1 |\V{c}^* \right)\\
  & \quad +  \mathbb{P}\left(\underset{q_1\in \{0,1\}, q_2 \in \{-B_1, B_1\}}{\max}
    \sum_{k=1}^K \left| \sum_{i=1}^N\sum_{j=1}^P\left(X_{ij} - \mathbb{E}(X_{ij}|\balp^*,\V{c}^*)\right)q_{jk}^cq_{ik}^{\alpha} \right|\epsilon_1
  \geq NP\epsilon |\V{c}^* \right)\\
  & \leq \sum_{j=1}^P\mathbb{P}\left( \left|\hat{\lambda}_j -\lambda_j^{*}\right| \geq \epsilon_1 |\V{c}^* \right)\\
  & \quad +   \sum_{k=1}^K\mathbb{P}\left(\underset{q_1\in \{0,1\}, q_2 \in \{-B_1, B_1\}}{\max}
    \left| \sum_{i=1}^N\sum_{j=1}^P\left(X_{ij} - \mathbb{E}(X_{ij}|\balp^*,\V{c}^*)\right)q_{jk}^cq_{ik}^{\alpha} \right|
  \geq \frac{NP\epsilon}{K\epsilon_1} |\V{c}^* \right)\\
  & \leq P^2C_1\exp(-C_2N\epsilon^2) + K2^{N+P} 2\exp(-\frac{NP^2\epsilon^2}{2(B_1K)^2\epsilon_1^2\sum_{j=1}^P\sigma_j^{*^2}}).
\end{align*}
}%

The third term (c) satisfies the inequality that

{\small
\begin{align*}
    & \mathbb{P}\left(\underset{q_1\in C_c, q_2 \in C_{\alpha}}{\max}
    \sum_{k=1}^K \left| \sum_{i=1}^N\sum_{j=1}^P\left((\hat{\lambda}_j-\lambda_j^*) \mathbb{E}(X_{ij}|\balp^*,\V{c}^*) \right)q_{jk}^cq_{ik}^{\alpha} \right|
  \geq NP\epsilon |\V{c}^* \right)\\
   & = \mathbb{P}\bigg(\underset{q_1\in C_c, q_2 \in C_{\alpha}}{\max}
    \sum_{k=1}^K \left| \sum_{i=1}^N\sum_{j=1}^P\left((\hat{\lambda}_j-\lambda_j^*) \mathbb{E}(X_{ij}|\balp^*,\V{c}^*) \right)q_{jk}^cq_{ik}^{\alpha} \right|
  \geq NP\epsilon, \\
  & \qquad \qquad \exists j, \left|\hat{\lambda}_j -\lambda_j^{*}\right| \geq \epsilon_1 |\V{c}^* \bigg) \\
  & \quad + \mathbb{P}\bigg(\underset{q_1\in C_c, q_2 \in C_{\alpha}}{\max}
    \sum_{k=1}^K \left| \sum_{i=1}^N\sum_{j=1}^P\left((\hat{\lambda}_j-\lambda_j^*) \mathbb{E}(X_{ij}|\balp^*,\V{c}^*) \right)q_{jk}^cq_{ik}^{\alpha} \right|
  \geq NP\epsilon,\\
  & \qquad \qquad  \forall j, \left|\hat{\lambda}_j -\lambda_j^{*}\right| < \epsilon_1 |\V{c}^* \bigg)\\
  & \leq \sum_{j=1}^P\mathbb{P}\left( \left|\hat{\lambda}_j -\lambda_j^{*}\right| \geq \epsilon_1 |\V{c}^* \right)\\
  & \quad + \mathbb{P}\left(\underset{q_1\in \{0,1\}, q_2 \in \{-B_1, B_1\}}{\max}
    \sum_{k=1}^K \left| \sum_{i=1}^N\sum_{j=1}^P\mathbb{E}(X_{ij}|\balp^*,\V{c}^*)q_{jk}^cq_{ik}^{\alpha} \right|\epsilon_1
  \geq NP\epsilon |\V{c}^* \right)\\
  & \leq  \sum_{j=1}^P\mathbb{P}\left( \left|\hat{\lambda}_j -\lambda_j^{*}\right| \geq \epsilon_1 |\V{c}^* \right)\\
  & \quad + 
  K2^N\mathbb{P}\left(\underset{q_1\in \{0,1\}}{\max}
    \left| \sum_{i=1}^N\sum_{j=1}^P\lambda_j^*\alpha_{ik}^*q_{jk}^c \right|
  \geq \frac{NP\epsilon}{B_1\epsilon_1} |\V{c}^* \right)\\
  & \leq  \sum_{j=1}^P\mathbb{P}\left( \left|\hat{\lambda}_j -\lambda_j^{*}\right| \geq \epsilon_1 |\V{c}^* \right)\\
  & \quad + 
  K2^N\mathbb{P}\left(\underset{q_1\in \{0,1\}}{\max}
    \left|\sum_{i=1}^N\alpha_{ik}^*\right| \left| \sum_{j=1}^P\lambda_j^*q_{jk}^c \right|
  \geq \frac{NP\epsilon}{B_1\epsilon_1} |\V{c}^* \right)\\
    & \leq  \sum_{j=1}^P\mathbb{P}\left( \left|\hat{\lambda}_j -\lambda_j^{*}\right| \geq \epsilon_1 |\V{c}^* \right)\\
  & \quad + 
  K2^N\mathbb{P}\left(
    \left|\sum_{i=1}^N\alpha_{ik}^*\right| PB_3/3
  \geq \frac{NP\epsilon}{B_1\epsilon_1} |\V{c}^* \right)\\
      & \leq  \sum_{j=1}^P\mathbb{P}\left( \left|\hat{\lambda}_j -\lambda_j^{*}\right| \geq \epsilon_1 |\V{c}^* \right)\\
  & \quad + 
  K2^N\mathbb{P}\left(
    \left|\sum_{i=1}^N\alpha_{ik}^*\right| 
  \geq \frac{3N\epsilon}{B_1B_3\epsilon_1} |\V{c}^* \right)\\
  & \leq 
  P^2C_1\exp(-C_2N\epsilon^2) + K2^N2\exp\left(-\frac{9N\epsilon^2}{2B_1^2B_3^2\epsilon_1^2\omega_{kk}}\right).
\end{align*}
}

Therefore,
\begin{align*}
   & \mathbb{P}\left(\underset{q_1\in C_c, q_2 \in C_{\alpha}}{\max}\left|\hat{J}_3(\bqc, \bqa; \hat{\Phi}) - \bar{J}_3(\bqc, \bqa; \Phi^*)\right|\geq NP\epsilon |\V{c}^* \right) \\
   & \leq \mathbb{P}\left(\underset{q_1\in C_c, q_2 \in C_{\alpha}}{\max}
    \sum_{k=1}^K \left| \sum_{i=1}^N\sum_{j=1}^P\left(\lambda_j^*X_{ij} -\lambda_j^*\mathbb{E}(X_{ij}|\balp^*,\V{c}^*) \right)q_{jk}^cq_{ik}^{\alpha}  \right|\geq NP\epsilon/3 |\V{c}^* \right)\\
    & \quad + \mathbb{P}\left(\underset{q_1\in C_c, q_2 \in C_{\alpha}}{\max}
    \sum_{k=1}^K \left| \sum_{i=1}^N\sum_{j=1}^P\left((\hat{\lambda}_j-\lambda_j^*)(X_{ij} - \mathbb{E}(X_{ij}|\balp^*,\V{c}^*))\right)q_{jk}^cq_{ik}^{\alpha} \right|
  \geq NP\epsilon/3 |\V{c}^* \right)\\
  & \quad + \mathbb{P}\left(\underset{q_1\in C_c, q_2 \in C_{\alpha}}{\max}
    \sum_{k=1}^K \left| \sum_{i=1}^N\sum_{j=1}^P\left((\hat{\lambda}_j-\lambda_j^*) \mathbb{E}(X_{ij}|\balp^*,\V{c}^*) \right)q_{jk}^cq_{ik}^{\alpha} \right|
  \geq NP\epsilon/3 |\V{c}^* \right)\\
  & \leq K2^{N+P} 2\exp(-\frac{NP^2\epsilon^2}{18(B_1K)^2\sum_{j=1}^P\lambda_j^{*2}\sigma_j^{*2}}) \\
  & \quad + P^2C_1\exp(-C_2N\epsilon^2/9) + K2^{N+P} 2\exp(-\frac{NP^2\epsilon^2}{18(B_1K)^2\epsilon_1^2\sum_{j=1}^P\sigma_j^{*^2}}) \\
  & \quad + P^2C_1\exp(-C_2N\epsilon^2/9) + K2^N2\exp\left(-\frac{N\epsilon^2}{2B_1^2B_3^2\epsilon_1^2\omega_{kk}}\right).
\end{align*}
Assume $\ln(P)/N = o(1)$ and take $\epsilon_1$ such that $\epsilon_1^2 < \frac{\epsilon^2}{2B_1^2B_3^2\omega_{kk}\ln2}$, the upper bound goes to zero as $N, P\longrightarrow \infty$.

The theorem follows from
\begin{align*}
    &\left|\hat{J}(\bqc, \bqa; \hat{\Phi}) - \bar{J}(\bqc, \bqa; \Phi^*)\right|\\
    \leq & \left|\hat{J}_1(\bqc, \bqa; \hat{\Phi}) - \bar{J}_1(\bqc, \bqa; \Phi^*)\right| + \left|\hat{J}_2(\bqc, \bqa; \hat{\Phi}) - \bar{J}_2(\bqc, \bqa; \Phi^*)\right| +\\
    & \left|\hat{J}_3(\bqc, \bqa; \hat{\Phi}) - \bar{J}_3(\bqc, \bqa; \Phi^*)\right| + \left|\hat{J}_4(\bqc, \bqa ; \hat{\Phi})\right|
\end{align*}
and $\underset{q_1\in C_c, q_2 \in C_{\alpha}}{\max}\left|\hat{J}_4(\bqc, \bqa ; \hat{\Phi})\right| = O(N+P)$. 
\end{proof}
%%%%%%%%%%%%%%%%%%%%%%%%%%%%%%%%%%%%%%%%%%%%%%%%%%%%%%%%%%%%%%%%%%%%%%%%%%%%%%

\subsubsection*{A7 Proof of Theorem 2}

\begin{theorem*}
Let $\eclass$ be the class of sets of elements that are equivalent to $(\bic, \balp^*, \Phi^*)$ up to community permutation. As $N,P \rightarrow \infty$ and $\log(P)/N = o(1)$, for all $\epsilon >0$,
\begin{align*}
    \mathbb{P}\left(d(\bic,\bqch)>\epsilon, \forall \bic \in \eclass |\V{c}^*\right) \longrightarrow 0,
\end{align*}
where $ d(\V{I}^c, \bqc) = \frac{1}{2P}\norm{\bic-\bqc}_1$ is the distance defined between $\V{I}^c$ and $\bqc$.
\end{theorem*}

\begin{proof}

{\small
\begin{align*}
    & \mathbb{P}\left(d(\bic,\bqch)>\epsilon, \forall \bic \in \eclass |c^*\right) \\
\leq & K!\mathbb{P}\left( d(\bic,\bqch)>\epsilon |c^*\right) \\
\leq & K!\mathbb{P}\left(\bar{J}(\bic, \balp^*) - \bar{J}(\bqch, \bqah) \geq \frac{PNm\gamma_1}{8}\epsilon|c^*\right) + o(1)\\
= & K!\mathbb{P}\left(\bar{J}(\bic, \balp^*) - \hat{J}(\bic, \balp^*) + \hat{J}(\bic, \balp^*) -\hat{J}(\bqch, \bqah) + \hat{J}(\bqch, \bqah) - \bar{J}(\bqch, \bqah) \geq \frac{PNm\gamma_1}{8}\epsilon|c^*\right) + o(1)\\
\leq & K!\mathbb{P}\left(\bar{J}(\bic, \balp^*) - \hat{J}(\bic, \balp^*) + \hat{J}(\bqch, \bqah) - \bar{J}(\bqch, \bqah) \geq \frac{PNm\gamma_1}{8}\epsilon |c^*\right)  + o(1)\\
\leq & K!\mathbb{P}\left(\bar{J}(\bic, \balp^*) - \hat{J}(\bic, \balp^*) \geq \frac{PNm\gamma_1}{16}\epsilon|c^*\right) \\
& + K!\mathbb{P}\left( \hat{J}(\bqch, \bqah) - \bar{J}(\bqch, \bqah) \geq \frac{PNm\gamma_1}{16} \epsilon|c^*\right)  + o(1).
\end{align*}
}
The theorem follows immediately from applying the theorem 1 on the last inequality.

\end{proof}
